# Supplementary material for: NeuralFuse: Learning to Recover the Accuracy of Access-Limited Neural Network Inference in Low-Voltage Regimes
Source: arXiv:2306.16869 source file (2024-12-12)
Supplement: Supplementary file 1 [file visualization_transformed_appendix_cifar100.tex]

\begin{figure*}[ht]
\centering
\captionsetup[subfigure]{font=large}
    \begin{adjustbox}{max width=\linewidth}
        \begin{tabular}{cc}
            \parbox[m]{1.5cm}{{\vspace{-9mm}\begin{flushright}Clean\end{flushright}}} &
            \includegraphics[width=.3\linewidth]{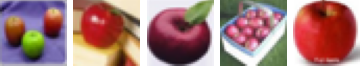} \\
            
            \parbox[m]{1.5cm}{{\vspace{-9mm}\begin{flushright}ConvL\end{flushright}}} &
            \includegraphics[width=.3\linewidth]{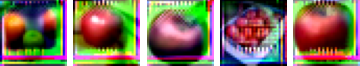} \\
            
            \parbox[m]{1.5cm}{{\vspace{-9mm}\begin{flushright}ConvS\end{flushright}}}&
            \includegraphics[width=.3\linewidth]{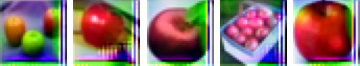} \\
            
            \parbox[m]{1.5cm}{{\vspace{-9mm}\begin{flushright}DeConvL\end{flushright}}}&
            \includegraphics[width=.3\linewidth]{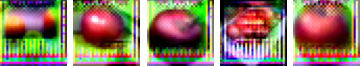} \\
            
            \parbox[m]{1.5cm}{{\vspace{-9mm}\begin{flushright}DeConvS\end{flushright}}}&
            \includegraphics[width=.3\linewidth]{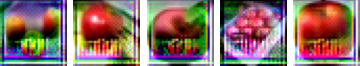} \\
            
            \parbox[m]{1.5cm}{{\vspace{-9mm}\begin{flushright}UNetL\end{flushright}}}&
            \includegraphics[width=.3\linewidth]{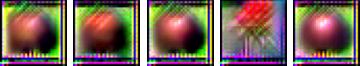} \\
            
            \parbox[m]{1.5cm}{{\vspace{-9mm}\begin{flushright}UNetS\end{flushright}}}&
            \includegraphics[width=.3\linewidth]{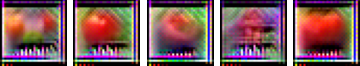} \\
        \end{tabular}
    \end{adjustbox}

\caption{Visualization results of the transformed images on CIFAR-100 from six different NeuralFuse generators trained with ResNet18 under $1\%$ of bit error rate.}
\label{fig:VisualizationImagesAppendixCifar100}
\end{figure*}
